# Supplementary material for: Weakly nonlinear rheology of transiently crosslinked biopolymer gels
Source: arXiv:1010.6264 source file (2010-10-29)
Supplement: Supplementary file 1 [file online_supplement.pdf]

# Online supplementary material to: Weakly nonlinear rheology of transiently crosslinked biopolymer gels

Lars Wolff*  Klaus Kroy*

October 29, 2010

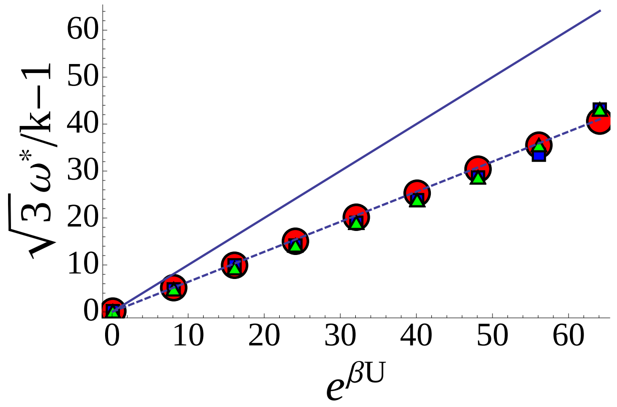


Figure 1: Frequency $\omega*$ of the absorption peak in dependence on the relative binding affinity $e^U$. Numerical evaluations of the inelastic power-law fluid for various values of $e^U$ and $\hat{f}\Delta x_b = 0.012$ (circles), 0.12 (squares), and 0.18 (triangles) compared to equations (17) (solid lines) and (18) (dashed lines) in the main text.

*Institute for Theoretical Physics, University of Leipzig, Germany

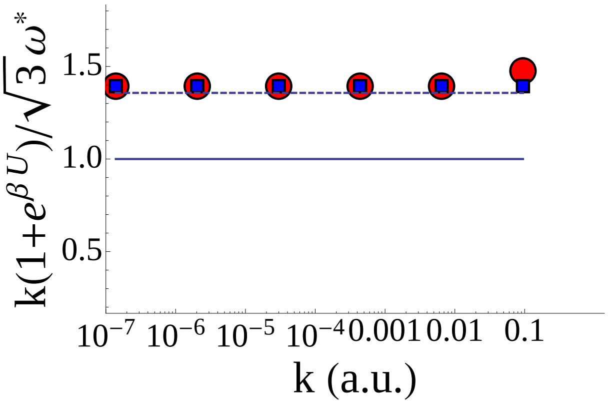


Figure 2: Position of the peak in the imaginary part of the nonlinear susceptibility. Numerical evaluations for the power-law fluid (blue squares) compared to numerical evaluations for the inelastic GWLC (red circles) and the analytical prediction, equation (17) in the main text (solid lines) and the semi-phenomenological correction, equation (18) in the main text (dashed lines), for various values of the equilibrium off rate $k$ ($10^{-8} < k < 0.1$). Here it was assumed that changing $k$ affects *via* the barrier height $\mathcal{E}$ the linear modulus of the GWLC (see section 3.2 in the main text). The driving amplitude was $\hat{f}\Delta x_b = 0.12$, other parameters as in figure 3 in the main text.
